# Supplementary material for: Freezing line of polydisperse hard spheres via direct-coexistence simulations
Source: arXiv:2505.14360 ancillary file (2025-10-08)
Supplement: Supplementary file 1 [file SM.pdf]

# Supplementary Material: Freezing line of polydisperse hard spheres via direct coexistence simulations

Antoine Castagnède,[1, a)] Laura Filion,[2] and Frank Smallenburg[1]
[1)] *Université Paris-Saclay, CNRS, Laboratoire de Physique des Solides, 91405 Orsay, France*
[2)] *Soft Condensed Matter and Biophysics, Debye Institute for Nanomaterials Science, Utrecht University, Utrecht, Netherlands*

## I. GENERATING A DETERMINISTIC GAUSSIAN SIZE DISTRIBUTION

We consider the freezing line of polydisperse mixtures in which the particle sizes follow a Gaussian distribution:

$$\mathcal{P}(\sigma) = \frac{1}{p\bar{\sigma}\sqrt{2\pi}} \exp\left[-\frac{1}{2}\left(\frac{\sigma-\bar{\sigma}}{p\bar{\sigma}}\right)^2\right]. \quad (1)$$

Here, $\bar{\sigma}$ is the mean particle diameter, and $p$ is the polydispersity, defined as the ratio between the standard deviation and the mean of the distribution.

To avoid any effects of randomness in the size distribution of the particles on simulations in the canonical ensemble, it is convenient to generate particle sizes deterministically. If we are generating $N$ particles according to a size distribution $P(\sigma)$, we can do this by generating sizes using the inverse cumulative distribution function $\Pi^{-1}(x)$, defined as the inverse of the cumulative distribution function

$$\Pi(\sigma) = \int_{-\infty}^{\sigma} \mathrm{d}x \mathcal{P}(x). \quad (2)$$

We can then choose

$$\sigma_i = \Pi^{-1}\left(\frac{i-1/2}{N}\right), \quad (3)$$

as our set of particle sizes, where $i = 1, ..., N$. For a Gaussian distribution with polydispersity $p$, this results in

$$\Pi(\sigma) = \frac{1}{2}\left(1 + \mathrm{Erf}\left(\frac{\sigma-\bar{\sigma}}{p\bar{\sigma}\sqrt{2}}\right)\right) \quad (4)$$

$$\Pi^{-1}(x) = \bar{\sigma}\left(1 + p\sqrt{2}\,\mathrm{Erf}^{-1}(2x-1)\right). \quad (5)$$

Note that due to the finite number of particles, this results in a distribution with a slightly lower polydispersity than $p$ for small systems. However, for a system of $N = 1000$ particles the relative deviation in $p$ is already on the order of $\sim 0.1\%$, and it further decreases (approximately $\propto 1/N$) for larger system sizes. Hence, we consider this deviation negligible.

[a)] **Author to whom correspondence should be addressed:** antoine.castagnede@universite-paris-saclay.fr

## II. POLYDISPERSE MIXTURES IN THE CANONICAL ENSEMBLE

In the canonical ensemble, a polydisperse system of particles is characterized by a fixed number of particles $N$, volume $V$, temperature $T$, and a size distribution $\{\sigma\}$. We can write the associated Helmholtz free energy as:

$$F(N,V,T,\{\sigma\}) = F_{\mathrm{mix}} + F_{\mathrm{conf}} \quad (6)$$

$$F_{\mathrm{conf}}(N,V,T,\{\sigma\}) = -k_B T \log Z_{\mathrm{conf}}(N,V,T,\{\sigma\}) \quad (7)$$

$$Z_{\mathrm{conf}}(N,V,T,\{\sigma\}) = \frac{1}{\Lambda^3 N!}\int \mathrm{d}\mathbf{r}^N \exp\left(-\beta U(\mathbf{r}^N,\{\sigma\})\right). \quad (8)$$

Here, $F_{\mathrm{mix}}$ and $F_{\mathrm{conf}}$ are the mixing and configurational parts of the free energy, respectively, $k_B$ is Boltzmann's constant, and $\beta = 1/k_B T$. Additionally, $U(\mathbf{r}^N,\{\sigma\})$ is the energy of a given configuration, and $\Lambda$ is the thermal wavelength.

For a macroscopic system ($N \to \infty$) with a size distribution $P(\sigma)$, we can define the mixing free energy by discretizing the size distribution[1]:

$$\beta F_{mix} = N \sum_i x_i \log x_i, \quad (9)$$

where

$$x_i = \mathcal{P}(i\lambda)\lambda \quad (10)$$

is the fraction of particles within some small interval $\lambda$ around a discretized size $\sigma_i^{\mathrm{disc}} = i\lambda$. In the limit of small intervals, this can also be written as:

$$\beta F_{mix} = N \int \mathrm{d}\sigma \mathcal{P}(\sigma) \log(\mathcal{P}(\sigma)\lambda). \quad (11)$$

Importantly, this mixing entropy is independent of the choice of $\lambda$ up to a constant shift in the free energy per particle, which will not influence phase behavior[1].

The chemical potential of a particle of size $\sigma_i$ is then defined as

$$\mu(\sigma_i) = \left(\frac{\partial F}{\partial N_i}\right)_{V,T,N_{j\neq i}} \quad (12)$$

$$= \mu_{mix}(\sigma_i) + \mu_{\mathrm{conf}}(\sigma_i). \quad (13)$$

Here, the mixing term $\mu_{mix}(\sigma_i)$ is given by

$$\mu_{mix}(\sigma_i) = k_B T \log x_i \quad (14)$$

$$= k_B T \log(\mathcal{P}(\sigma_i)\lambda). \quad (15)$$

Note that similar to the free energy, a change in $\lambda$ only results in a trivial shift in the chemical potential, which again does not influence phase behavior. For the purpose of this paper, we will simply set $\lambda$ equal to the average particle size in the fluid phase $\bar{\sigma}$.

## III. MEASURING RELATIVE CHEMICAL POTENTIALS

We would like to measure the relative chemical potential function $\delta\mu(\sigma)$ in a simulation in the canonical ensemble. Here, $\delta\mu(\sigma) = \mu(\sigma) - \mu(\sigma_{\text{ref}})$ is the chemical potential of a particle of size $\sigma$ relative to that of a particle of an arbitrary reference size $\sigma_{\text{ref}}$. To this end, we first consider how changing the size of a single particle changes the canonical free energy of the system.

### A. Effect of changing one particle's size on the free energy

We can now consider the effect of a change to the size of particle $i$, such that its size changes from $\sigma_i$ to $\sigma_i + \epsilon$. This affects both the mixing free energy and the configurational part. The total change in free energy can be written as:

$$\Delta F = \Delta F_{mix} + \Delta F_{\text{conf}}. \tag{16}$$

Note that $\Delta F$ can also be regarded as the effect of taking out a particle of size $\sigma_i$ and putting in a particle of size $\sigma_i + \epsilon$. In other words,

$$\Delta F = \mu(\sigma_i + \epsilon) - \mu(\sigma_i). \tag{17}$$

For the mixing free energy, we can simply consider removing a particle of size $\sigma_i$ and inserting a particle of size $\sigma_i + \epsilon$. Using the mixing part of the chemical potential, this yields:

$$\beta\Delta F_{mix} = \beta\mu_{mix}(\sigma_i + \epsilon) - \beta\mu_{mix}(\sigma_i). \tag{18}$$

For the configurational part of the free energy:

$$\beta\Delta F_{\text{conf}} = -\log\frac{\int \mathrm{d}\mathbf{r}^N \exp\left(-\beta U(\mathbf{r}^N, \{\tilde{\sigma}\})\right)}{\int \mathrm{d}\mathbf{r}^N \exp\left(-\beta U(\mathbf{r}^N, \{\sigma\})\right)}, \tag{19}$$

where $\{\tilde{\sigma}\}$ is the set of particle sizes after the change. We can rewrite the numerator:

$$\begin{aligned}\beta\Delta F_{\text{conf}} &= -\log\frac{\int \mathrm{d}\mathbf{r}^N \exp(-\beta\Delta U)\exp\left(-\beta U(\mathbf{r}^N, \{\sigma\})\right)}{\int \mathrm{d}\mathbf{r}^N \exp\left(-\beta U(\mathbf{r}^N, \{\sigma\})\right)}, \\ &= -\log\left\langle \exp(-\beta\Delta U)\right\rangle_{\{\sigma\}}, \end{aligned}\tag{20}$$

where $\Delta U$ is the change in potential energy due to the change in the size of particle $i$, and the subscript on the angular brackets indicates that the ensemble average is taken at the original distribution of sizes $\{\sigma\}$. For hard spheres, $\Delta U$ is either infinite or zero, depending on whether the particle size change creates an overlap, and hence $\exp(-\beta\Delta U)$ evaluates to either 0 or 1.

We now consider an infinitesimal change to the size of particle $i$, by taking the limit $\epsilon \to 0$. From Eq. 17, we obtain:

$$\frac{\partial F}{\partial \sigma_i} = \mu'(\sigma_i) = \delta\mu'(\sigma_i). \tag{21}$$

Additionally, from Eqs. 18 and 20, we obtain:

$$\frac{\partial F}{\partial \sigma_i} = \mu'_{mix}(\sigma_i) + \left\langle \frac{\partial U}{\partial \sigma_i}\right\rangle. \tag{22}$$

Since $\mu'_{\text{mix}}$ is known from the size distribution, we can determine the derivative of the chemical potential $\delta\mu'(\sigma_i)$ for any particle size, by measuring the ensemble average $\left\langle \frac{\partial U}{\partial \sigma_i}\right\rangle$ for different particle sizes $\sigma_i$. Subsequently, $\delta\mu(\sigma_i)$ can be trivially obtained by integrating $\delta\mu'(\sigma_i)$. For continuous potentials, $\left\langle \frac{\partial U}{\partial \sigma_i}\right\rangle$ can be measured straightforwardly. However, since our system of interest consists of hard spheres, the energy of the system is not a continuously differentiable function of the particle sizes, and slightly more care needs to be taken to measure $\delta\mu$.

### B. Measuring $\delta\mu(\sigma)$ for hard spheres

The hard-sphere pair potential depends on the particle sizes as

$$U_{ij}(\mathbf{r}_{ij}, \sigma_i, \sigma_j) = \tilde{U}^{\text{HS}}\left(r_{ij} - \frac{\sigma_i}{2} + \frac{\sigma_j}{2}\right). \tag{23}$$

Hence, it is more convenient to work in terms of the radius $R_i = \sigma_i/2$ of the particle than the diameters:

$$\frac{\partial U}{\partial \sigma_i} = 2\frac{\partial U}{\partial R_i} = -2\langle f_{R_i}\rangle, \tag{24}$$

where $f_{R_i}$ is the force experienced by the radius of particle $i$. We can write this average as a time-average:

$$\begin{aligned} f_{R_i} &= \frac{-1}{t_b - t_a}\int_{t_a}^{t_b} \mathrm{d}t \sum_j \frac{\partial U_{ij}}{\partial R_i} && (25)\\ &= \frac{-1}{t_b - t_a}\int_{t_a}^{t_b} \mathrm{d}t \sum_j |\mathbf{f}_{ij}| && (26)\\ &= \frac{-1}{t_b - t_a}\sum_c m|\left(\delta\mathbf{v}_i\right)_c|, && (27)\end{aligned}$$

Here, $\mathbf{f}_{ij}(t) = -\frac{\partial U_{ij}}{\partial \mathbf{r}_{ij}}$ is the force on particle $i$ due to particle $j$. We have used the fact that the hard-sphere potential is repulsive (i.e. $\frac{\partial U_{ij}}{\partial \sigma_i} \geq 0$) and acts along the radius of each particle. In the last step, $(\delta\mathbf{v}_i)_c$ is the change in velocity of particle $i$ during collision $c$, $m$ is mass of a particle (taken equal for all particles), and the sum is taken over all collisions in the time interval $[t_a, t_b]$.

## IV. POLYDISPERSE MIXTURES WITH DYNAMIC PARTICLE SIZES

We are interested in the equilibrium behavior of polydisperse mixtures in three dimensions. For our direct coexistence simulations, it is helpful to consider these systems in the semi-grand-canonical ensemble, i.e. at constant number of particles $N$, volume $V$, temperature $T$, and relative size-dependent chemical potential $\delta\mu(\sigma)$. Analogous to the "continuous time swap" approach of Ref. 2, we can consider the semigrand ensemble as a description of a system where each particle has three positional degrees of freedom and one for its radius. The Hamiltonian for this system can then be written as:

$$H = \sum_i \left[ \frac{p_i^2}{2m_i} + \frac{\wp_i^2}{2M} + V(R_i) \right] + \sum_{i<j} U_{ij}(\mathbf{r}_{ij}, R_i, R_j), \quad (28)$$

where $\mathbf{p}_i$ is the translational momentum of particle $i$ with mass $m$, $\wp_i$ is the momentum associated with its radius $R_i$, $M$ is the corresponding mass, $V(R_i) = -\delta\mu(\sigma_i = 2R_i)$ is the external field controlling the particle sizes, $U_{ij}$ represents the pair interaction, and $\mathbf{r}_{ij}$ is the vector connecting particles $i$ and $j$.

The canonical partition function for this system can then be written as

$$Z(N, V, T, \delta\mu(\sigma)) = \frac{1}{h^{4N} N!} \int \mathrm{d}\mathbf{r}^N \mathrm{d}\mathbf{p}^N \mathrm{d}\sigma^N \mathrm{d}\wp^N \exp\left(-\beta H\right), \quad (29)$$

where $h$ is a discretization constant used to ensure $Z$ is dimensionless, and $\beta = 1/k_B T$ with $k_B$ Boltzmann's constant. Integrating out the (translational and size) momenta yields:

$$Z = \frac{1}{\Lambda^{3N} \lambda^N N!} \int \mathrm{d}\mathbf{r}^N \mathrm{d}R^N \exp\left( -\beta \sum_{i<j} U_{ij} \right) \times \exp\left( \beta \sum_i \delta\mu(R_i) \right), \quad (30)$$

where $\Lambda = h/\sqrt{2\pi m k_B T}$ is the usual thermal wavelength, $\lambda = h/\sqrt{2\pi M k_B T}$ is its analogue for the size degree of freedom. Note that apart from the irrelevant prefactor $1/\lambda^N$, this corresponds to the semigrand-canonical partition function that one would obtain for a system which can swap particles (at fixed total $N$) with an external particle reservoir where the chemical potential of a particle of size $\sigma$ is given by $\delta\mu(\sigma) + c$, where $c$ is an arbitrary constant. Hence, a simulation in the canonical ensemble governed by the Hamiltonion in Eq. 28 will correctly sample the semigrand ensemble governed only by the particle interactions and an imposed relative chemical potential $\delta\mu(\sigma)$.

For systems with continuous interaction potentials, the Hamiltonian in Eq. 28 gives rise to equations of motion that can be directly implemented in standard (time-driven) molecular dynamics schemes. However, for hard spheres, the interaction potential is discontinuous, and hence we will use event-driven simulations instead.

This poses two problems. First, we will need to derive a collision rule for our variable-size particles, which will update not only the translational velocities of the colliding particles, but also their size velocities $\dot{\sigma}_i$. Second, we need to predict and handle "collisions" with the external potential $V(\sigma_i)$, which will affect only the radial velocities of the particles. We will discuss these two topics in the following two subsections.

### A. Pair collision rules

For a pair potential of the form $U_{ij} = U(r_{ij} - R_i - R_j)$, the Hamiltonian in Eq. 28 gives rise to the following equations of motion:

$$\dot{\mathbf{r}}_i = \frac{\partial H}{\partial \mathbf{p}_i} = \mathbf{p}_i/m_i \quad (31)$$

$$\dot{R}_i = \frac{\partial H}{\partial \wp_i} = \wp_i/M \quad (32)$$

$$\dot{\mathbf{p}}_i = -\frac{\partial H}{\partial \mathbf{r}_i} = \sum_{i \neq j} \mathbf{f}_{ij} \quad (33)$$

$$\dot{\wp}_i = -\frac{\partial H}{\partial R_i} = -V'(R_i) + \sum_{i \neq j} \mathbf{f}_{ij} \cdot \hat{\mathbf{r}}_{ij}. \quad (34)$$

During a pair collision, the changes in $\dot{\mathbf{p}}_i$ and $\dot{\wp}_i$ are fully dominated by the pairwise forces, and hence the effects of the external field $V$ can be ignored. To determine the collision rule, we can regularize the interaction as

$$U_{ij}(\mathbf{r}_i, \mathbf{r}_j, R_i, R_j) = -\frac{\xi(\mathbf{r}_{ij}, R_i, R_j)}{\epsilon} \Theta(-\xi(\mathbf{r}_{ij}, R_i, R_j)), \quad (35)$$

where

$$\xi(\mathbf{r}_{ij}, R_i, R_j) = |\mathbf{r}_{ij}| - R_i - R_j \quad (36)$$

is the surface-to-surface distance between the spheres, $\Theta$ is the Heaviside step function, and $\mathbf{r}_{ij} = \mathbf{r}_i - \mathbf{r}_j$. This continuous pair potential represents a short-range repulsion for overlapping particles ($\xi < 0$), which converges to the hard-sphere potential in the limit $\epsilon \to 0$. The equations of motion for the velocities during the collision then become:

$$\dot{\mathbf{p}}_1 = \Theta(-\xi) \frac{\hat{\mathbf{r}}_{12}}{\epsilon} \quad (37)$$

$$\dot{\mathbf{p}}_2 = -\Theta(-\xi) \frac{\hat{\mathbf{r}}_{12}}{\epsilon}. \quad (38)$$

$$\dot{\wp}_i = -\frac{\Theta(-\xi)}{\epsilon} \quad (39)$$

During the collision, i.e. during the period where $\xi < 0$, we obtain:

$$\dot{\xi} = \mathbf{v}_{12} \cdot \hat{\mathbf{r}}_{12} - \frac{\wp_1 + \wp_2}{M} \quad (40)$$

$$\ddot{\xi} = \frac{2}{\epsilon} \left( \frac{1}{m} + \frac{1}{M} \right) + \mathbf{v}_{12} \cdot \frac{\partial \hat{\mathbf{r}}_{12}}{\partial t} \quad (41)$$

In the limit of small $\epsilon$, we can neglect the last term in $\ddot{\xi}$. The acceleration is then constant during the collision, and we can solve for the total duration of the collision:

$$\Delta t = \frac{\dot{\xi}(t = t_{col})}{\ddot{\xi}(t = t_{col})} = \epsilon \frac{b(t_{col})}{\frac{1}{m} + \frac{1}{M}}, \quad (42)$$

where

$$b(t) = \mathbf{v}_{12}(t) \cdot \mathbf{r}_{12}(t) - \frac{\wp_1(t) - \wp_2(t)}{M} \quad (43)$$

is the surface-to-surface velocity of the two particles along the $\hat{\mathbf{r}}_{12}$ direction, which we evaluate at the time $t_{col}$ where the collision starts. The change in momenta is then given by

$$\Delta \mathbf{p}_1 = \frac{b(t_{col})\hat{\mathbf{r}}_{12}}{\frac{1}{m} + \frac{1}{M}} \quad (44)$$

$$\Delta \mathbf{p}_2 = -\frac{b(t_{col})\hat{\mathbf{r}}_{12}}{\frac{1}{m} + \frac{1}{M}} \quad (45)$$

$$\Delta \wp_i = \frac{b(t_{col})}{\frac{1}{m} + \frac{1}{M}}. \quad (46)$$

Note that this result is independent of $\epsilon$ and hence also holds in the limit of $\epsilon \to 0$, where the collision becomes a hard-core collision. This gives us a set of collision rules for polydisperse hard spheres of variable size. These rules conserve the translational momentum and the total kinetic energy (translational + radial) of the system.

The introduction of the radial "mass" $M$ introduces a free parameter into the simulation, given by $\alpha = m/M$. Low $\alpha$ (high $M$) will result in relatively slower motion of the particle sizes. The choice of $\alpha$ should not affect any static equilibrium properties (including phase behavior) of the system, but will influence dynamics. As the growing and shrinking of particles is not physical anyway, we arbitrarily set $\alpha = 1$.

Finally, we note that predicting the collision time for hard spheres with a constant radial velocity is largely analogous to predicting collisions of hard spheres of constant size. Specifically, it involves solving a quadratic equation

$$|\mathbf{r}_{ij}(t)|^2 = \sigma_{ij}(t)^2, \quad (47)$$

with $\sigma_{ij}(t) = R_i(t) + R_j(t)$ the time-dependent contact distance between the two spheres. Since both sides of the equation can be written as second-order polynomials of $t$, this can be analytically solved for $t$, yielding:

$$t_{\text{col}} - t_{\text{current}} = \frac{-b - \sqrt{b^2 - a(r_{ij}^2 - \sigma_{ij}^2)}}{a}, \quad (48)$$

$$a = (v_{ij}^2 + \dot{\sigma}_{ij}^2), \quad (49)$$

where all time-dependent quantities are evaluated at the current simulation time $t_{\text{current}}$. Note that future collisions only occur when $b < 0$ or $a < 0$, and additionally the discriminant (inside the square root) is larger than zero. Otherwise, no future collisions are expected.

## B. Collision rules with the field $V(R)$

Traditionally, event-driven simulations are commonly used for potentials and energy fields that are piecewise constant functions, such as hard spheres or other shapes, square-well interactions, and systems of these particles interacting with with hard walls or external stepwise potential fields. For these types of systems, the momentum of a particle only changes at discrete events in time. However, in the canonical ensemble, continuous potentials can also be addressed using an event-driven approach. Specifically, Peters and De With[3] have introduced a rejection free event-driven Monte Carlo (EDMC) algorithm for simulating particles with continuous interaction potentials. In this approach, the interaction between pairs of particles gives rise to stochastic collisions, with the collision distance determined based on a random number drawn from a Boltzmann distribution at the imposed temperature $T$. Between these collisions, the particles experience free flight as normal in an event-driven molecular dynamics (EDMD) simulation. As a result, it has been shown that the EDMC approach can be an efficient alternative to conventional MD simulations in the canonical ensemble, assuming the interaction potential is short-ranged and easily invertible[4].

Here, we adapt this approach to handle the effects of the field $V(R)$ that controls the size distribution of the particles. Specifically, whenever we predict the next collision for a given particle, we also consider the possibility of colliding with the field $V(R)$. To this end, we draw a random energy $\Delta V$ from a Boltzmann distribution, and we find the radius $R_{\text{col}}$ such that the total increase in energy encountered between the current particle radius $R(t)$ and $R_{\text{col}}$ is equal to $\Delta V$. As proven in Ref. 3, this approach will correctly sample the canonical ensemble.

In practice, our function $V(R)$ is taken to be a cubic polynomial (which we find fits our data for $\delta\mu(\sigma)$ excellently, see main text). Additionally, we only allow $R$ to vary within a region $[R_{\text{min}}, R_{\text{max}}]$ of permitted values, chosen large enough to ensure that the probability of hitting either edge is negligible. Moreover, we find that $V(R)$ is always either a monotonically decreasing function of $R$ or has a single minimum at $R_{\text{well}}$ (and no maximum) within the allowed region. We therefore have to consider three cases (see Fig. 1):

1. The particle's radius is going "uphill" (i.e. $V(R)$ is increasing as a function of time). An example is shown in Fig. 1a for a shrinking particle. In this case, the particle is allowed to continue going uphill until an amount of energy equal to $\Delta V$ has been expended. In other words, the radius at which the collision with the field occurs is such that $V(R_{\text{col}}) = V_{\text{col}} = V(R) + \Delta V$, with $R$ the current particle radius. If this radius lies outside the interval $[R_{\text{min}}, R_{\text{max}}]$, the collision occurs at the edge of this interval, instead. For a growing particle whose radius starts off larger than $R_{\text{well}}$, the procedure is

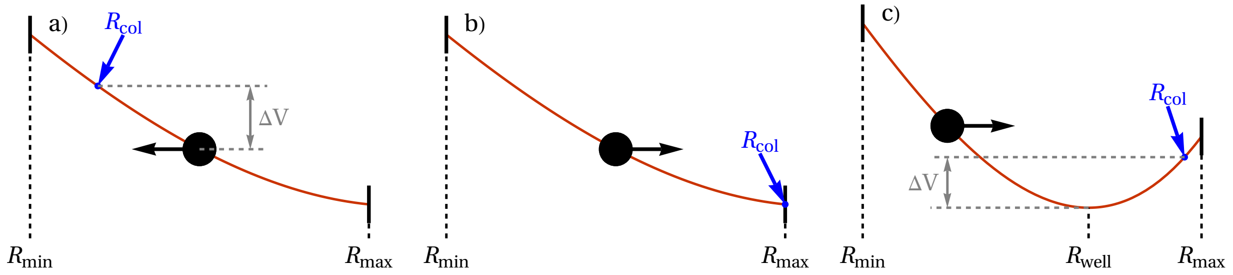


FIG. 1. Illustration of the prediction of particle-field collisions in the semigrand-canonical ensemble simulations. The solid red lines depict the field $V(R)$ felt by the particle's radius. The black dot and arrow denote the particle's current radius and whether the particle is currently growing or shrinking. The blue dot denotes the predicted value of $R$ at the moment of collision (which may depend on the stochastically chosen value of $\Delta V$). The three depicted cases correspond to a) uphill motion, b) downhill motion without a minimum, and c) downhill motion with a minimum.

exactly the same.

2. The particle's radius is going "downhill" (i.e. $V(R)$ is decreasing as a function of time), and will reach an edge of $[R_{\rm min}, R_{\rm max}]$ before encountering a local minimum. For our systems, this only applies to growing particles (Fig. 1b). The field collision is then scheduled at $R_{\rm col} = R_{\rm max}$.

3. The particle's radius is going downhill towards the minimum in $V(R)$ at $R_{\rm well}$. In this case, we ignore the downhill part of the trajectory, and we find the collision radius corresponding to $V(R_{\rm col}) = V_{\rm col} = V(R_{\rm well}) + \Delta V$. In other words, $\Delta V$ now measures the permitted increase in energy starting from the minimum[3] (Fig. 1c). Again, if the collision radius falls outside $[R_{\rm min}, R_{\rm max}]$, the collision occurs at the edge of this interval instead.

Finally, for all three cases described above, once $R_{\rm col}$ is determined, the associated collision time can be trivially determined as $(R_{\rm col} - R)/\dot{R}$, making use of the fact that $\dot{R}$ is constant between collisions.

Note that since our expression for $V(R)$ is a cubic polynomial with real coefficients, solving $V(R_{\rm col}) = V_{\rm col}$ can be done analytically. This is done by transposing $V(R)$ into a depressed cubic of the form $t^3 + pt + q = 0$ (with $p$ and $q$ constants), and expressing the real roots using hyperbolic or trigonometric functions depending on their multiplicity. For more complex forms of $V(r)$, numerical root-finding methods or lookup tables would likely be necessary.

## V. SYSTEM SIZE EFFECTS

We show in Fig. 2 the effect of system size on the determination of the coexistence pressure for hard spheres with a polydispersity of $p = 0.06$. As one might expect, larger systems lead to less noise. However, the obtained coexistence pressures are not strongly affected by system size.

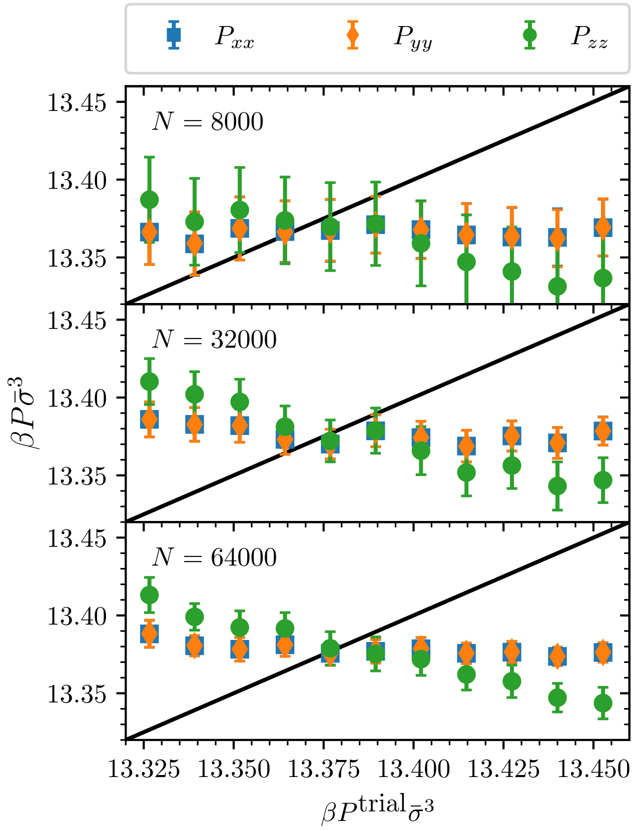


FIG. 2. Pressure tensor components $P_{xx}$, $P_{yy}$, and $P_{zz}$ as a function of trial pressure $P^{\rm trial}$ obtained from semi-grand direct coexistence simulations for system with 16000 particles, polydispersity $p = 0.06$, and varying system size. Error bars show one standard error. These systems were set so the fluid–crystal interface corresponds to the square lattice plane of an FCC crystal.

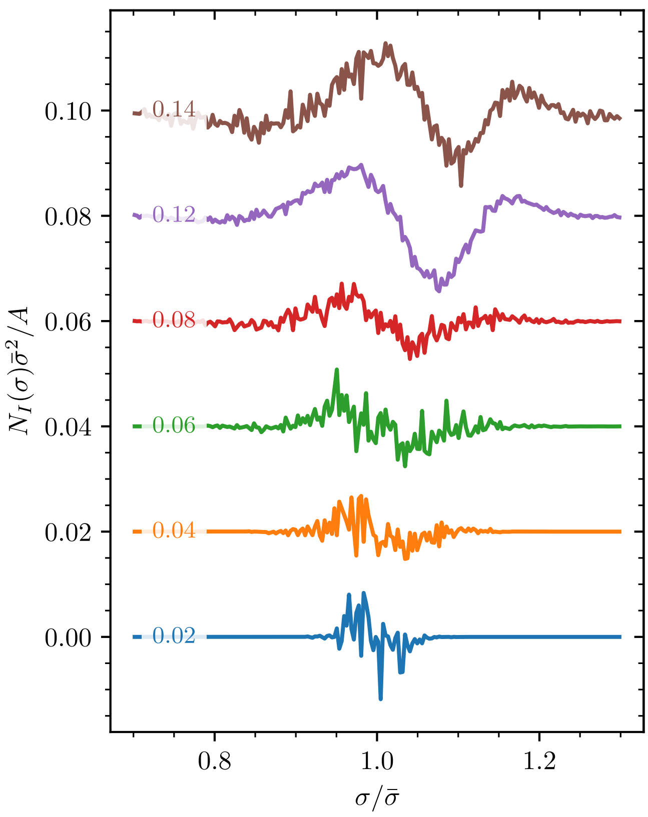


FIG. 3. Surface excess concentration of particles per unit area with size $\sigma_i$ for an equimolar Gibbs dividing surface in a system with 16384 particles at coexistence. Here the crystal orientation is such that the hexagonal FCC planes are parallel to the elongated dimension of the simulation box ($FCC_b$). Polydispersities are reported on each line, all lines are vertically shifted for readability.

## VI. PHASE COMPOSITION AND EXCESS SURFACE ABSORPTION AT COEXISTENCE

Fig. 3 shows the excess surface absorption for the $FCC_b$ interface. Additionally, we show in Fig. 4 the particle size distribution at coexistence in the fluid phase, FCC phase, and coexisting system ($FCC_a$ interface) for each of the investigated polydispersities. We note that the behavior of the the coexisting system with $FCC_b$ interface is qualitatively very similar.

## VII. REFERENCES

[1]Daan Frenkel. Why colloidal systems can be described by statistical mechanics: some not very original comments on the gibbs paradox. *Mol. Phys.*, 112(17):2325–2329, 2014.

[2]Ludovic Berthier, Elijah Flenner, Christopher J Fullerton, Camille Scalliet, and Murari Singh. Efficient swap algorithms for molecular dynamics simulations of equilibrium supercooled liquids. *J. Stat. Mech.: Theory Exp.*, 2019(6):064004, 2019.

[3]Elias AJF Peters and G de With. Rejection-free monte carlo sampling for general potentials. *Phys. Rev. E*, 85(2):026703, 2012.

[4]Antoine Castagnède, Laura Filion, and Frank Smallenburg. Fast event-driven simulations for soft spheres: from dynamics to laves phase nucleation. *J. Chem. Phys.*, 161(2):024116, 2024.

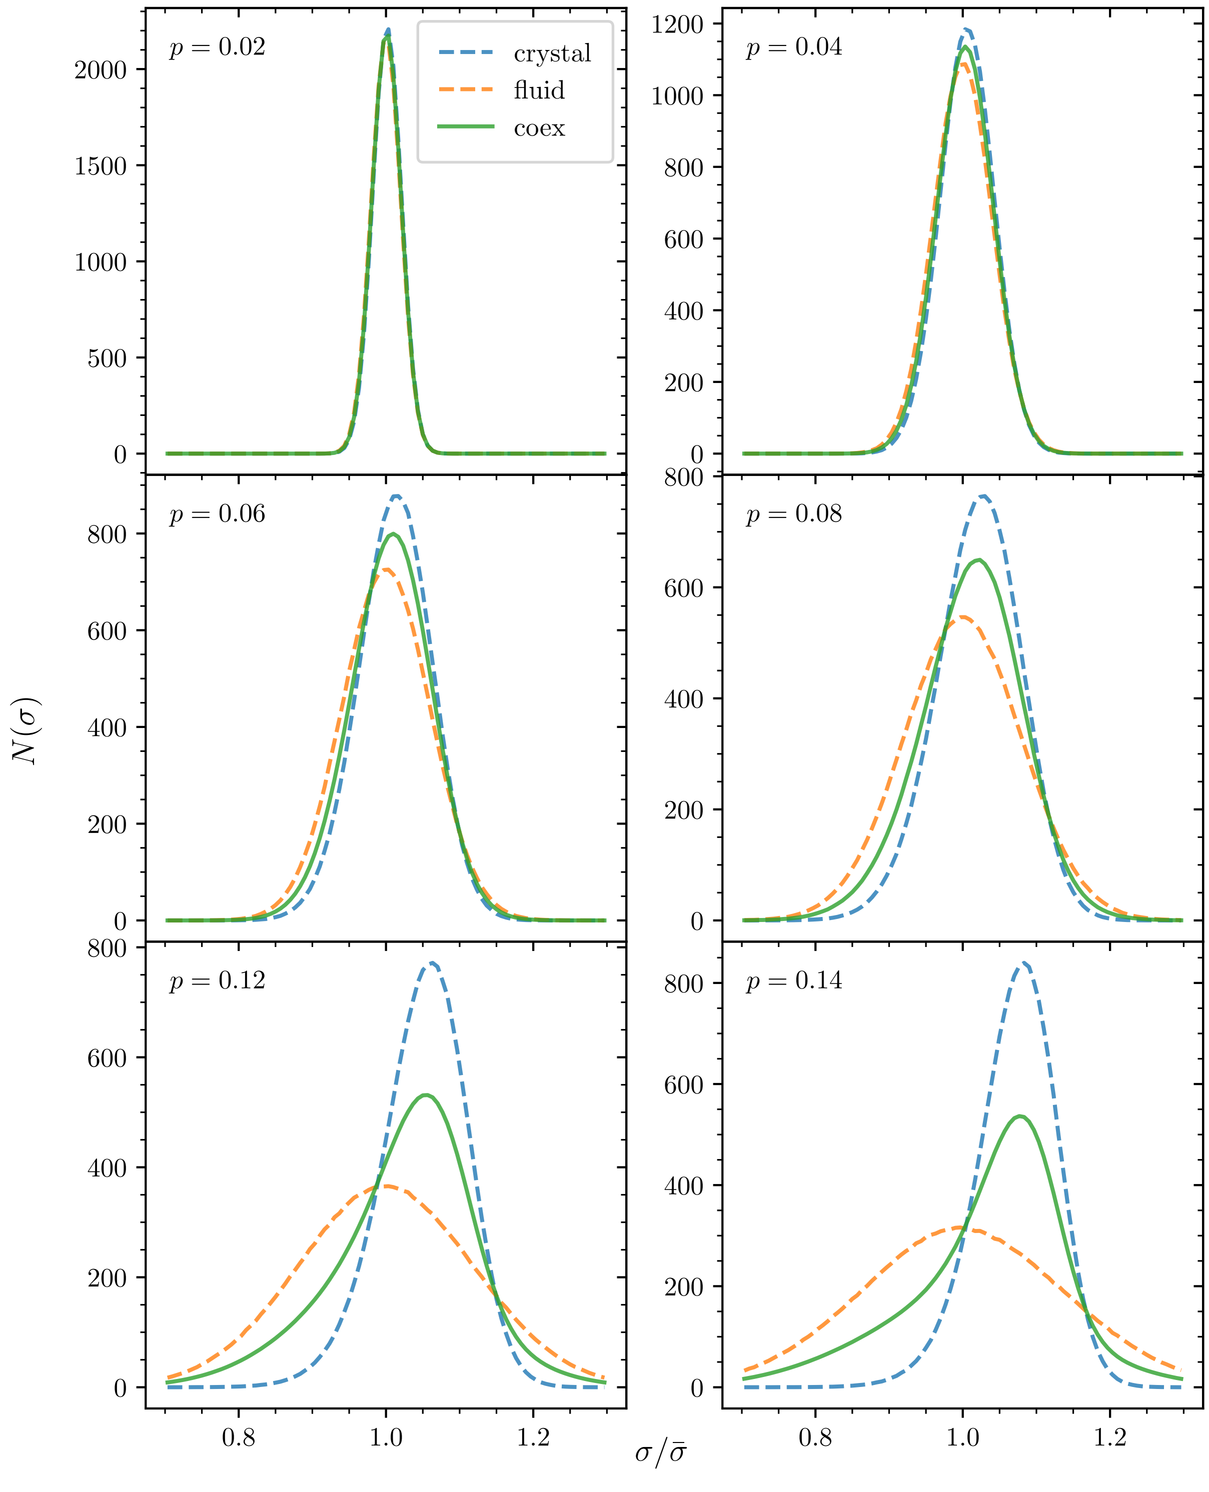


FIG. 4. Particle size distribution of direct coexistence simulations ($FCC_a$ interface, solid green lines) for the range of polydispersities explored in this work. In each direct coexistence simulation, the global density was chosen to be exactly halfway between the fluid and crystal coexistence densities. Also shown are the compositions of the bulk coexisting fluid (dashed orange lines) and crystal (dashed blue lines) phases.
